# Supplementary material for: Many Hands Make Light Work: Using Essay Traits to Automatically Score Essays
Source: arXiv:2102.00781 source file (2021-02-01)
Supplement: Supplementary file 1 [file Supplementary.tex]

\newpage
\appendix
\newpage

\begin{table*}[t]
\centering
\resizebox{\textwidth}{!}{%
\begin{tabular}{|l|l|c|c|c|c|c|c|c|c|c|c|}
\hline
\textbf{Essay Set} & \textbf{System} & \textbf{Cont.} & \textbf{Org.} & \textbf{WC} & \textbf{SF} & \textbf{Conv.} & \textbf{PA} & \textbf{Lang.} & \textbf{Narr.} & \textbf{Style} & \textbf{Voice}\\ \hline
\multirow{4}{*}{Prompt 1} & Random Forest & 0.628 & 0.606 & 0.618 & 0.594 & 0.588 & --- & --- & --- & --- & --- \\
 & Kernel & \textit{0.686} & \textit{0.637} & \textit{0.659} & \textit{0.639} & \textit{0.620} & --- & --- & --- & --- & --- \\
 & STL-LSTM & \textbf{0.703} & \textbf{0.664} & \textbf{0.675} & \textbf{0.648} & \textbf{0.638} & --- & --- & --- & --- & --- \\
 & MTL-BiLSTM & 0.663 & 0.631 & 0.648 & 0.633 & 0.612 & --- & --- & --- & --- &  --- \\\hline
\multirow{4}{*}{Prompt 2} & Random Forest & 0.563 & 0.551 & 0.531 & 0.495 & 0.486 & --- & --- & --- & --- & --- \\
 & Kernel & 0.600 & 0.570 & 0.583 & 0.544 & 0.530 & --- & --- & --- & --- & --- \\
 & STL-LSTM & \textbf{0.617} & \textbf{0.623} & \textbf{0.630} & \textbf{0.603} & \textbf{0.601} & --- & --- & --- & --- & --- \\ 
 & MTL-BiLSTM & \textit{0.608} & \textit{0.572} & \textit{0.611} & \textit{0.597} & \textit{0.591} & --- & --- & --- & --- & --- \\ \hline
\multirow{4}{*}{Prompt 3} & Random Forest & 0.586 & --- & --- & --- & --- & 0.575 & 0.534 & 0.594 & --- & --- \\
 & Kernel & \textit{0.659} & ---  & --- & --- & --- & \textit{0.658} & \textit{0.590} & 0.645 & --- & --- \\
 & STL-LSTM & \textbf{0.673} & --- & --- & --- & --- & \textbf{0.683} & \textbf{0.612} & \textbf{0.684} & --- & --- \\
 & MTL-BiLSTM & 0.645 & --- & --- & --- & --- & 0.649 & 0.588 & \textit{0.666} & --- & --- \\\hline
\multirow{4}{*}{Prompt 4} & Random Forest & 0.646 & --- & --- & --- & --- & 0.636 & 0.577 & 0.641 & --- & --- \\
 & Kernel & 0.702 & ---  & --- & --- & --- & 0.702 & 0.571 & 0.687 & --- & --- \\
 & STL-LSTM & \textbf{0.751} & --- & --- & --- & --- & \textbf{0.738} & \textbf{0.645} & \textbf{0.722} & --- & --- \\
 & MTL-BiLSTM & \textit{0.742} & --- & --- & --- & --- & \textit{0.723} & \textit{0.588} & \textit{0.689} & --- & --- \\\hline
\multirow{4}{*}{Prompt 5} & Random Forest & 0.667 & --- & --- & --- & --- & 0.639 & 0.618 & 0.647 & --- & --- \\
 & Kernel & 0.713 & ---  & --- & --- & --- & \textit{0.700} & 0.620 & 0.635 & --- & --- \\
 & STL-LSTM & \textbf{0.738} & --- & --- & --- & --- & \textbf{0.719} & \textbf{0.638} & \textbf{0.700} & --- & --- \\
 & MTL-BiLSTM & \textit{0.717} & --- & --- & --- & --- &    0.698 & \textbf{0.638} & \textit{0.667} & --- & --- \\\hline
\multirow{4}{*}{Prompt 6} & Random Forest & 0.579 & --- & --- & --- & --- & 0.581 & 0.555 & 0.592 & --- & --- \\
& Kernel & 0.759 & --- & --- & --- & --- & \textit{0.727} & \textit{0.638} & \textit{0.667} & --- & --- \\
 & STL-LSTM & \textbf{0.820} & --- & --- & --- & --- & \textbf{0.783} & \textbf{0.664} & \textbf{0.690} & --- & --- \\
 & MTL-BiLSTM & \textit{0.766} & --- & --- & --- & --- & 0.723 & 0.600 & 0.648 & --- & ---\\\hline
\multirow{4}{*}{Prompt 7} & Random Forest & 0.495 & 0.528 & --- & --- & 0.533 & --- & --- & --- & 0.577 & --- \\
 & Kernel & 0.737 & \textit{0.659} & --- & --- & 0.504 & --- & --- & --- & 0.609 & --- \\
 & STL-LSTM & \textbf{0.771} & \textbf{0.676} & --- & --- & \textbf{0.621} & --- & --- & --- & \textbf{0.659} & --- \\
 & MTL-BiLSTM & \textit{0.766} & \textit{0.659} & --- & --- & \textit{0.569} & --- & --- & --- & \textit{0.632} & --- \\\hline
\multirow{4}{*}{Prompt 8} & Random Forest & 0.510 & 0.571 & 0.518 & 0.507 & 0.431 & --- & --- & --- & --- & 0.507 \\
 & Kernel & \textit{0.573} & 0.572 & 0.494 & 0.477 & 0.455 & --- & --- & --- & --- & 0.489 \\
 & STL-LSTM & \textbf{0.586} & \textbf{0.632} & \textbf{0.559} & \textbf{0.586} & \textbf{0.558} & --- & --- & --- & --- & \textit{0.544} \\ 
 & MTL-BiLSTM & 0.569 & \textit{0.599} & \textit{0.585} & \textit{0.565} & \textit{0.467} & --- & --- & --- & --- & \textbf{0.582} \\ \hline
\multirow{4}{*}{\textbf{Mean QWK}} & Random Forest & 0.584 & 0.564 & 0.556 & 0.532 & 0.510 & 0.608 & 0.571 & 0.619 & 0.577 & 0.507 \\
 & Kernel & 0.679 & 0.610 & 0.579 & 0.553 & 0.527 & 0.693 & \textit{0.605} & 0.651 & 0.609 & 0.489 \\
 & STL-LSTM & \textbf{0.707} & \textbf{0.649} & \textbf{0.621} & \textbf{0.612} & \textbf{0.605} & \textbf{0.731} & \textbf{0.640} & \textbf{0.699} & \textbf{0.659} & \textit{0.544} \\ 
 & MTL-BiLSTM & \textit{0.685} & \textit{0.615} & \textit{0.615} & \textit{0.598} & \textit{0.560} & \textit{0.698} & 0.604 & \textit{0.668} & \textit{0.632} & \textbf{0.582} \\\hline
\end{tabular}%
}
\caption{Results of the String Kernel system of \cite{cozma-etal-2018-automated} and the best STL system \cite{dong-etal-2017-attention} compared with our MLT-BiLSTM system. The  ``---'' denotes that the particular trait is not applicable for that particular essay set. The different traits are Content (Cont.), Organization (Org.), Word Choice (WC), Sentence Fluency (SF), Conventions (Conv.), Prompt Adherence (PA), Language (Lang.), Narrativity (Narr.), Style and Voice. The last set of rows, \textbf{Mean QWK} is the mean QWK predicted for all the traits across all the eight essay sets. The best results are marked in \textbf{boldface}, and the second-best results are marked in \textit{italics}.}
\label{Traits Results Table}
\end{table*}

\section{Supplementary Material}

\subsection{Auxiliary Task Results}

Table \ref{Traits Results Table} is the results for the trait scores predictions for the different systems, namely Random Forest \cite{mathias-bhattacharyya-2018-asap}, String Kernel \cite{cozma-etal-2018-automated}, the best STL system \cite{dong-etal-2017-attention} and our best MTL system.
